# Supplementary material for: Disguise without Disruption: Utility-Preserving Face De-Identification
Source: arXiv:2303.13269 source file (2023-12-18)
Supplement: Supplementary file 1 [file tab-supp-gauslaplac.tex]

\begin{table}[t]
% \vspace{-1.8em}
\centering
\caption{\bpnote{Finalize and discuss table. (or remove?)} \zikui{It is fine removing it. In the supp, maybe do not resize tables to unify font sizes across tables}}
\label{tab:supp-gauslapla}
% \resizebox{\linewidth}{!}{
    \begin{tabular}{c|cc|cc}
    \toprule
    \multicolumn{1}{c|}{\multirow{3}[4]{*}{\makecell{Noise \\ Level}}} & \multicolumn{4}{c}{TPR (\%) @ FPR=1e-3 $\downarrow$ (LFW data)} \\
\cmidrule{2-5}          & \multicolumn{2}{c|}{Swapped} & \multicolumn{2}{c}{Inverted} \\
          & Gaussian & Laplacian & Gaussian & Laplacian \\
    \midrule
    $\beta=1.0$     & 0.03  & 0.2   & 13    & 20.4 \\
    $\beta=1.5$   & 0.07  & 0.2   & 9.37  & 15.9 \\
    $\beta=2.0$     & 0.37  & 0.3   & 7.43  & 14.2 \\
    $\beta=2.5$   & 0.33  & 0.3   & 6.5   & 12.4 \\
    $\beta=3.0$     & 0.37  & 0.3   & 5.37  & 12.1 \\
    \bottomrule
\end{tabular}
% }
% \vspace{-1.1em}
% \vspace{-1.8em}
\end{table}
